# Supplementary material for: Lattice model for percolation on a plane of partially aligned sticks with length dispersity
Source: arXiv:2405.13728 ancillary file (2024-08-08)
Supplement: Supplementary file 1 [file SM.pdf]

**Lattice model for percolation on a plane of partially aligned sticks with length dispersity**
**Supplemental Material**

Avik P. Chatterjee[1,2*] and Yuri Y. Tarasevich[3]

[1] Department of Chemistry, SUNY-ESF, One Forestry Drive, Syracuse, NY 13210, USA
[2]The Michael M. Szwarc Polymer Research Institute, Syracuse, NY 13210, USA
[3] Institute of Physics, Fluminense Federal University, Niterói, Brazil

The effect of partial alignment upon the percolation threshold for monodisperse sticks for the stepfunction angular PDF (PDF A) is shown in Fig. S1. The computer simulation study [1] reported that for this choice of PDF: (i) $\rho_c L^2$ depended only weakly upon the cutoff angle $\alpha$ for $\alpha \geq 5\pi/18$, but that (ii) for $\alpha < 5\pi/18$ the threshold increased with the degree of alignment, approximately following: $\rho_c L^2 \sim \alpha^{-0.9}$. Our results are qualitatively similar to these findings with the distinction that Eqn. (28) in main text predicts that for small values of $\alpha$ (high degrees of alignment), $\rho_c L^2 \approx 1/\alpha$ instead. The dotted and dashed lines in Fig. S1 denote the behaviors $\rho_c L^2 \approx 1/\alpha$ and $\rho_c L^2 \approx 1/\alpha^{0.9}$, respectively. Given the similarity between the curves it could be difficult to distinguish between these values for the apparent exponent especially for a limited range of $\alpha$.

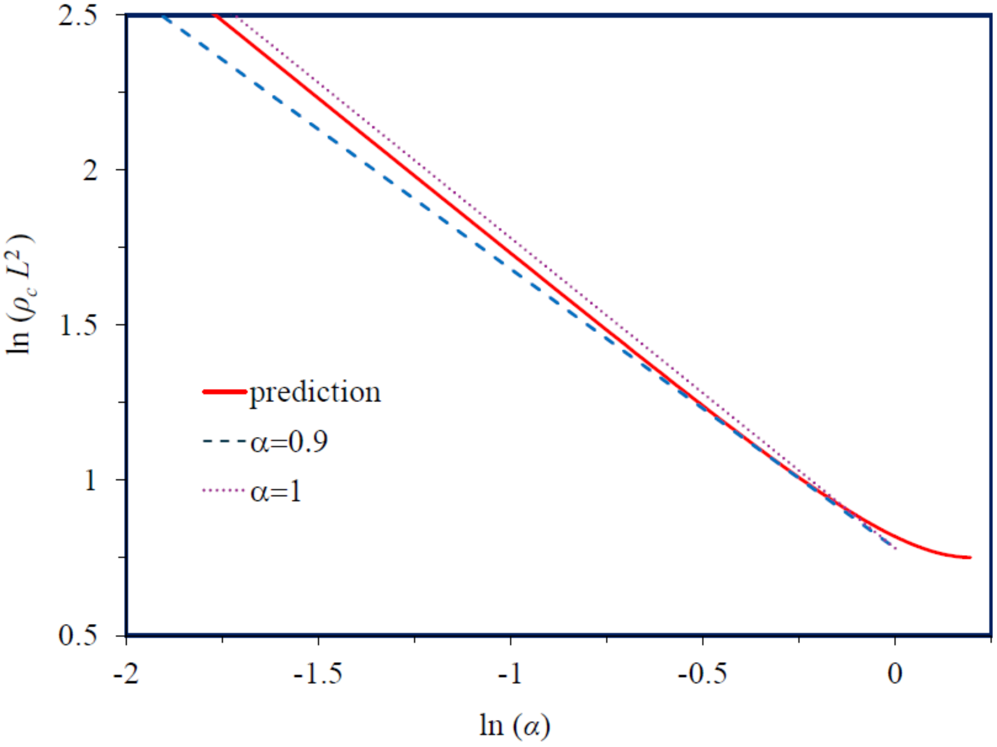


**Fig. S1.** The solid line depicts the percolation threshold for monodisperse, partially aligned sticks calculated from (28) in main text for PDF A (16) in main text as a function of the cutoff angle $\alpha$. The dotted and dashed lines in Fig. S1 depict the behaviors $\rho_c L^2 \approx 1/\alpha$ and $\rho_c L^2 \approx 1/\alpha^{0.9}$, respectively.

The combined and simultaneous effects of both polydispersity and alignment upon the percolation threshold have been examined in the simulation study reported in [2] which investigated a log-normal distribution over stick lengths and a Gaussian distribution (PDF B in the present account) over stick angular orientations. Figure S2 depicts the dependence of $\rho_c\langle L\rangle^2$ upon polydispersity in the stick lengths for various prescribed, fixed value of the order parameter $S$. The solid, dashed, and dotted lines represent calculations from our model using PDFs B, C, and D, respectively. For each set of curves (including the symbols that represent simulation results from [2] from top to bottom, $S = 0.9$, 0.5, and 0 (isotropic), respectively. Increasing the polydispersity in stick lengths (quantified by $\sigma_L/\langle L\rangle$) for a fixed value of $S$ always lowers the threshold, while increasing the degree of alignment for a given distribution over stick lengths has the opposite effect. Results from the simulations of [2] are in close agreement with those obtained from our model using the same PDF (PDF B). The sensitivity of the predicted values of $\rho_c\langle L\rangle^2$ to the choice of angular PDF for high degrees of stick alignment is clearly seen in the substantial difference between the dotted and dashed curves, which represent respectively maximal and minimal variances in orientational angle that are consistent with a prescribed value of $S$. For the calculations depicted in Figs. S2 and S3 that employ the Gaussian PDF (PDF B), the quantity $\langle|\sin\gamma|\rangle$ required in evaluating the right-hand-side of (27) in main text is obtained by numerical integration.

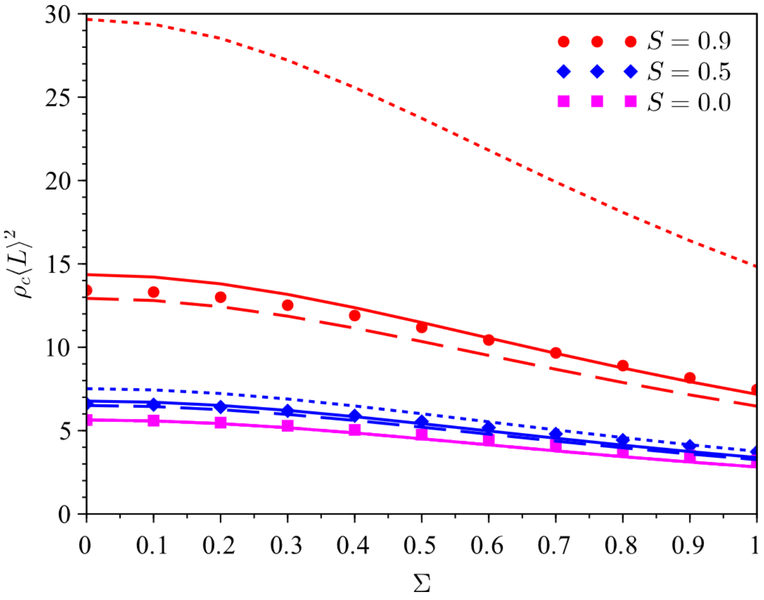


**Fig. S2.** The percolation threshold $\rho_c\langle L\rangle^2$ is shown as a function of the degree of polydispersity in the lengths of the sticks ($\sigma_L/\langle L\rangle$) for fixed values of the orientational order parameter $S$. The diamonds, squares, and triangles represent the simulation results from [2] for values of $S$ equal to 0.9, 0.5, and 0 (isotropic), respectively. The solid, dashed, and dotted lines represent calculations from our model (27) in main text using PDFs B, C, and D, respectively. For each of these sets of curves, the value of $S$ is equal to 0.9, 0.5, and 0, respectively, from top to bottom. The dotted, dashed, and solid lines coincide for the case that $S = 0$.

The dependence of $\rho_c\langle L\rangle^2$ upon the extent of alignment (quantified by $S$) for various fixed degrees of polydispersity ($\sigma_L/\langle L\rangle$) is shown in Fig. S3. Consistent with the findings depicted in Fig. 1, the threshold is seen to increase steeply with increasing degrees of alignment especially for

large values of $S$, while polydispersity in the stick lengths lowers the critical value of $\rho\langle L\rangle^2$. Results from our Gaussian PDF (PDF B) (the solid lines in Fig. S3) are similar to those reported in [2]. (It should be noted that in our model $\rho_c\langle L\rangle^2$vanishes in the limits that either (i) $\langle L^2\rangle/\langle L\rangle^2 \rightarrow \infty$, or (ii) $S \rightarrow$ zero.) Increasing polydispersity at a fixed value of $\langle L\rangle$ implies the presence of increasing fractions of longer sticks that have a higher likelihood to cross and form contacts, thereby lowering the areal number density at the threshold.

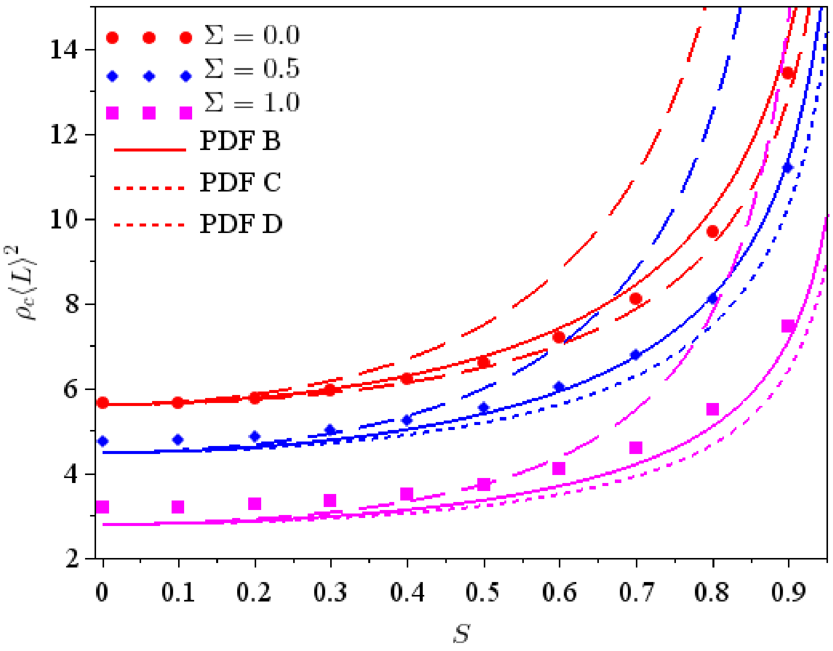


**Fig. S3.** The percolation threshold $\rho_c\langle L\rangle^2$ is shown as a function of the degree of alignment ($S$) of the sticks for fixed values of the polydispersity in stick lengths ($\sigma_L/\langle L\rangle$). The diamonds, squares, and triangles represent the simulation results from [2] for values of $\sigma_L/\langle L\rangle$ equal to 1.0, 0.5, and 0 (monodisperse), respectively. The solid, dashed, and dotted lines represent calculations from our model (27) in main text using PDFs B, C, and D, respectively. For each of these sets of curves, the value of $\sigma_L/\langle L\rangle$ is equal to 0 (monodisperse), 0.5, and 1.0, respectively, from top to bottom.

## References


[1] S.-H. Yook, W. Choi, and Y. Kim, Conductivity of stick percolation clusters with anisotropic alignments, J. Korean Phys. Soc. 61, 1257 (2012).

[2] Y. Y. Tarasevich and A. V. Eserkepov, Percolation of sticks: Effect of stick alignment and length dispersity, Phys. Rev. E 98, 062142 (2018).
